# Supplementary material for: Cosine Model Watermarking Against Ensemble Distillation
Source: arXiv:2203.02777 source file (2022-03-05)
Supplement: Supplementary file 1 [file appendix.tex]

% !TEX root = ../main.tex
\clearpage
\appendix
\begin{center}
{\Large \bf Appendix}
\end{center}
%\par\noindent\rule{\textwidth}{1pt}
\setcounter{section}{0}
In this appendix, we provide the proofs for Theorem 1 in Section~\ref{proof}. In addition, we show more extensive experimental results in Section \ref{supexp}.

\section{Proofs}
\subsection{Proof of Theorem \ref{bound}}\label{proof}
\begin{proof}
We first prove the left inequality of \eqref{eq:bound}. By using the triangular inequality and the fact that $\mathbf{s}^*(\bar{D})$
is the best sinusoidal fit for $\bar{D}$, we have
\begin{align*}
    \chi^2_f(D) & \geq \sum_{l=1}^L \left[ \mathbf{\bar q}^l_{i^*} -[\mathbf{s}^*(D)]_l \right]^2 - \sum_{l=1}^L \left[ \mathbf{\bar q}^l_{i^*} -\mathbf{q}^l_{i^*} \right]^2 \\
    &  \geq \sum_{l=1}^L \left[ \mathbf{\bar q}^l_{i^*} -[\mathbf{s}^*(\bar{D})]_l \right]^2 - L_{SE} \\
   &  = {\chi}^2_f(\bar{D})  - L_{SE}.
\end{align*}
Combining the above inequality with equation (\ref{eq:LSdef}) we have the left inequality of \eqref{eq:bound} hold.

Next we prove the right inequality of \eqref{eq:bound}. Since $\mathbf{s}^*(\hat{D})$ and $\mathbf{s}^*(\tilde{D})$ are 
the points from sinusoidal functions with same frequency $f$, then
$\frac{1}{N}\mathbf{s}^*(\hat{D}) +  \frac{N-1}{N}\mathbf{s}^*(\tilde{D})$ is also a set of points from a sinusoidal function. As $\mathbf{s}^*(D)$
is the best sinusoidal fit for $D$, we have
\begin{align*}
   \chi^2_f (D) & = \sum_{l=1}^L \left[ \mathbf{q}^l_{i^*} - [{\mathbf{s}}^*(D)]_l \right]^2 \\
& \leq \sum_{l=1}^L \left[ \mathbf{q}^l_{i^*} - \left[\frac{1}{N}\mathbf{s}^*(\hat{D}) +  \frac{N-1}{N}\mathbf{s}^*(\tilde{D})\right]_l \right]^2. 
\end{align*}
By using the above inequality and triangular inequality, we have following inequality:

\begin{align*}
    &\chi^2_f (D)  \leq \sum_{l=1}^L \left[ \mathbf{q}^l_{i^*} - \frac{1}{N}[ \mathbf{s}^*(\hat{D})]_l -  \frac{N-1}{N}[\mathbf{s}^*(\tilde{D})]_l \right]^2\\
    & \leq \sum_{l=1}^L \left[ \mathbf{q}^l_{i^*} - \frac{1}{N}\hat{\mathbf{q}}^l_{i^*} - \frac{N-1}{N}\mathbf{\tilde q}^l_{i^*} \right]^2 +\\
    & \quad \sum_{l=1}^L \left[ \frac{1}{N}\hat{\mathbf{q}}^l_{i^*} + \frac{N-1}{N}\mathbf{\tilde q}^l_{i^*} - \frac{1}{N}[ \mathbf{s}^*(\hat{D})]_l - \frac{N-1}{N}[ \mathbf{s}^*(\tilde{D})]_l \right]^2\\
& \leq L_{SE} + \\
& \sum_{l=1}^L \left[ \frac{1}{N}\left[\hat{\mathbf{q}}^l_{i^*} - [ \mathbf{s}^*(\hat{D})]_l\right]+ \frac{N-1}{N}\left[\mathbf{\tilde q}^l_{i^*}  - [ \mathbf{s}^*(\tilde{D})]_l\right] \right]^2\\
    & \leq L_{SE} +  \frac{1}{N^2} {\chi}^2_f(\hat{D}) + \left(\frac{N-1}{N}\right)^2{\chi}^2_f((\tilde{D}).
\end{align*}
Combining the above inequality with equation (\ref{eq:LSdef}) we have the right inequality of \eqref{eq:bound} hold.

\end{proof}

\subsection{Lemma 1: Modified Softmax Properties}
\label{proof-lemma}
\begin{lem}
\label{lemma-1}
Let $\mathbf{q}$ be the softmax output of a model $R$, then the modified softmax $\hat{\mathbf{q}}$, as defined in \eqref{eq:modified_softmax} satisfies Property \ref{prop:softmax}.
\end{lem}

\begin{proof}
    for all $i$ we have 
    \begin{gather*}
        0 \leq \mathbf{q}_i \leq 1,\\
        -1 \leq \mathbf{a}_i(\mathbf{x}) \leq 1.
    \end{gather*}
    Therefore, when $i = i^*$, we have
    \begin{equation*}
        0 \leq \mathbf{q}_i + \varepsilon (1 + \mathbf{a}_i(\mathbf{x})) \leq 1 + 2 \varepsilon,
    \end{equation*}
    and then 
   \begin{equation*}
      0 \leq \frac{\mathbf{q}_i + \varepsilon (1 + \mathbf{a}_i(\mathbf{x}))}{1 + 2 \varepsilon} \leq 1. 
   \end{equation*}
    When $i \neq i^*$, since $m\geq 2$, we have
    \begin{equation*}
         0 \leq \mathbf{q}_i + \frac{\varepsilon (1 + \mathbf{a}_i(\mathbf{x}))}{m - 1} \leq 1 + \frac{2 \varepsilon}{m-1} \leq 1 + 2 \varepsilon,
    \end{equation*}
    and then
    \begin{equation*}
       0 \leq \frac{\mathbf{q}_i + \frac{\varepsilon (1 + \mathbf{a}_i(\mathbf{x}))}{m - 1}}{1 + 2 \varepsilon} \leq 1. 
    \end{equation*}
    Thus, $\hat{\mathbf{q}}$ satisfies clause 1 of Property \ref{prop:softmax}.
    
    To prove the clause 1 of Property \ref{prop:softmax}, we use the fact that $\mathbf{a}_{i^*} + \mathbf{a}_{j \neq i^*} = 0$ and get
    \begin{align*}
        \sum_i^m \hat{\mathbf{q}}_i &= \frac{\mathbf{q}_{i^*} + \varepsilon(1 + \mathbf{a}_{i^*})}{1 + 2\varepsilon} + \sum_{j \neq i^*} \frac{\mathbf{q}_{j} + \frac{\varepsilon(1 + \mathbf{a}_j)}{m-1}}{1 + 2\varepsilon}\\
        & = \left(\sum_{j=1}^m \frac{\mathbf{q}_i}{1 + 2 \varepsilon}\right) + \left(\sum_{j\neq i^*} \frac{\varepsilon (1 + \mathbf{a}_{i^*} + 1 + \mathbf{a}_{j \neq i^*})}{(m-1)(1 + 2 \varepsilon)}\right)\\
        & = \frac{1}{1 + 2 \varepsilon}  + \frac{2 \varepsilon}{1 + 2 \varepsilon}\\
        & = 1.
    \end{align*}
    Thus, clause  2 of Property \ref{prop:softmax} is also satisfied.
\end{proof}

\section{More experiments}
\label{supexp}
\subsection{Results for FMNIST}
\label{appx:extra}
Results for FMNIST

\subsection{Teacher Ensemble Size Analysis}
\label{appx:ens_size_graphs}

\chu{Analyze the influence of parameters on the performance of our method.}

We analyze the effect of the the teacher ensemble size value to DeepMark's performance.
In general the watermark of a teacher model will be more diluted in the ensemble model's outputs the more models are present in the ensemble.
Therefore we expect all methods to decrease in performance as the ensemble size increase.

\begin{figure}%
    \centering
    \includegraphics[width = 0.42\textwidth]{figures/map_size_cifar10}
    \caption{Mean average precision of different watermarking methods and Fingerprinting under different parameter values as a function of ensemble size.
    Each watermarked model was part of an ensemble of teacher models and was the only watermarked model within that ensemble.}
    \label{fig:map_vs_size_1wm}
\end{figure}
    
\begin{figure}%
    \centering
    \includegraphics[width = 0.42\textwidth]{figures/map_size_cifar10_all_wm}
    \caption{Mean average precision of different watermarking methods and Fingerprinting under different parameter values as a function of ensemble size.
    Each watermarked model was part of an ensemble of teacher models and was the only watermarked model within that ensemble.}
    \label{fig:map_vs_size_awm}
\end{figure}

Figures \ref{fig:map_vs_size_1wm} and \ref{fig:map_vs_size_awm} show the mAP as a function of ensemble sizes for DeepMark, DAWN, and Fingerprint, for different watermark parameter values for DeepMark and DAWN.
For all methods and parameter values, the watermark performance generally decreases as the ensemble size increases.
However, except for the smallest value of $\varepsilon=0.025$, DeepMark's performance is generally superior for larger ensembles, and decreases more gradually than DAWN and Fingerprinting.

\subsection{Signal Frequency Analysis}
\label{appx:frequency}

\subsection{Experiments with True Labels}
\label{appx:truelabel}
